# Supplementary material for: Parameter Estimation-Based Extended Observer for Linear Systems with Polynomial Overparameterization
Source: arXiv:2302.13705 ancillary file (2024-02-13)
Supplement: Supplementary file 1 [file supp.pdf]

# Supplement to "Parameter Estimation-Based Extended Observer for Linear Systems with Polynomial Overparametrization"

Anton Glushchenko, *Member, IEEE* and Konstantin Lastochkin

**Abstract**

This article is a supplementary material for "Parameter Estimation-Based Extended Observer for Linear Systems with Polynomial Overparametrization" by the same authors. It provides proofs of Lemma 1, Lemma 2 and Theorem, as well as the description of the system for the numerical experiments.

## I. Proof of Lemma 1 in the Manuscript

***Lemma 1.*** *Let $t_\epsilon > t_0$ be a sufficiently large predefined time instant, then for all $t \ge t_\epsilon$ the unknown parameters $\eta(\theta)$ and unmeasured states $\xi(t)$ satisfy the following regression models:*

$$\begin{gathered}\mathcal{Y}(t) = \Delta(t)\,\eta(\theta),\\ \mathcal{Y}(t) = k(t)\cdot \operatorname{adj}\{\varphi(t)\}\,q(t),\ \Delta(t) = k(t)\cdot\det\{\varphi(t)\},\end{gathered}$$

$$\begin{gathered}\xi(t) = z(t) + R^{\mathrm{T}}(t)\,\kappa(\theta),\\ \kappa(\theta) = \begin{bmatrix}\psi_a^{\mathrm{T}}(\theta) & \psi_b^{\mathrm{T}}(\theta) & \psi_d^{\mathrm{T}}(\theta)\end{bmatrix}^{\mathrm{T}},\\ R^{\mathrm{T}}(t) = \begin{bmatrix}\Omega(t) & P(t) & U(t)\end{bmatrix},\end{gathered}$$

*where*

$$\begin{gathered}q(t) = \int\limits_{t_\epsilon}^{t} e^{-\sigma(\tau - t_\epsilon)}\overline{\varphi}_f(\tau)\left(\ \overline{q}(\tau) - k_1\overline{q}_f(\tau) - \beta^{\mathrm{T}}\left(F_f(\tau) + l y_f(\tau)\right)\ \right)d\tau,\ q(t_\epsilon) = 0_{2n},\\ \varphi(t) = \int\limits_{t_\epsilon}^{t} e^{-\sigma(\tau - t_\epsilon)}\overline{\varphi}_f(\tau)\,\overline{\varphi}_f^{\mathrm{T}}(\tau)\,d\tau,\ \varphi(t_\epsilon) = 0_{2n\times 2n},\end{gathered}$$

$$\begin{gathered}\dot{\overline{q}}_f(t) = -k_1\overline{q}_f(t) + \overline{q}(t),\ \overline{q}_f(t_0) = 0,\\ \dot{\overline{\varphi}}_f(t) = -k_1\overline{\varphi}_f(t) + \overline{\varphi}(t),\ \overline{\varphi}_f(t_0) = 0_{2n},\\ \dot{F}_f(t) = -k_1 F_f(t) + F(t),\ F_f(t_0) = 0_{n_\delta},\\ \dot{y}_f(t) = -k_1 y_f(t) + y(t),\ y_f(t_0) = 0,\end{gathered}$$

$$\begin{gathered}\overline{q}(t) = y(t) - C_0^{\mathrm{T}}z,\ \overline{\varphi}(t) = \begin{bmatrix}\dot{\Omega}^{\mathrm{T}}C_0 + N^{\mathrm{T}}\beta\\ \dot{P}^{\mathrm{T}}C_0 + H^{\mathrm{T}}\beta\end{bmatrix},\\ \dot{z}(t) = A_K z(t) + K y(t),\ z(t_0) = 0_n,\\ \dot{\Omega}(t) = A_K\Omega(t) + I_n y(t),\ \Omega(t_0) = 0_{n\times n},\\ \dot{P}(t) = A_K P(t) + I_n u(t),\ P(t_0) = 0_{n\times n},\end{gathered}$$

$$\begin{gathered}\dot{U}(t) = A_K U(t) + I_n\delta(t),\ U(t_0) = 0_{n\times n},\\ \dot{F}(t) = GF(t) + Gly(t) - lC_0^{\mathrm{T}}\dot{z}(t),\ F(t_0) = 0_{n_\delta},\\ \dot{H}(t) = GH(t) - lC_0^{\mathrm{T}}\dot{P}(t),\ H(t_0) = 0_{n_\delta\times n},\\ \dot{N}(t) = GN(t) - lC_0^{\mathrm{T}}\dot{\Omega}(t),\ N(t_0) = 0_{n_\delta\times n},\end{gathered}$$

*and, if $\overline{\varphi}(t) \in \mathrm{FE}$ over $[t_\epsilon; t_e]$, then for all $t \ge t_e$ it holds that $\Delta_{\max} \ge \Delta(t) \ge \Delta_{\min} > 0$.*

*Here $k(t) > k_{\min} > 0$ is a time-varying (or time-invariant) amplifier, $k_1 > 0$, $\sigma > 0$ are filters time constants, $A_K = A_0 - KC_0^{\mathrm{T}}$, $G$ stand for stable matrices of appropriate dimensions, $l \in \mathbb{R}^{n_\delta}$ denotes a vector such that the pair $(G, l)$ is controllable, and $G$ is chosen so as to satisfy the condition $\sigma\{\mathcal{A}_\delta\} \cap \sigma\{G\} = 0$, $\beta \in \mathbb{R}^{n_\delta}$ is a solution of the following set of equations:*

$$\begin{gathered}M_\delta\mathcal{A}_\delta - GM_\delta = l\overline{h}_\delta^{\mathrm{T}},\ \overline{h}_\delta^{\mathrm{T}} = h_\delta^{\mathrm{T}}\mathcal{A}_\delta,\\ \beta = \overline{h}_\delta^{\mathrm{T}}M_\delta^{-1}.\end{gathered}$$

*Proof:* The parametrization (11) is obtained by combining the results of [S1, S2] with the dynamic regressor extension and mixing procedure. The proof of Lemma 1 is derived on the basis of the results of Lemma 1 and Theorem 2 from [S2].

A. Glushchenko is with V.A. Trapeznikov Institute of Control Sciences of Russian Academy of Sciences, Moscow, Russia aiglush@ipu.ru
K. Lastochkin is with V.A. Trapeznikov Institute of Control Sciences of Russian Academy of Sciences, Moscow, Russia lastconst@ipu.ru

To make it easier to understand the notation and to ensure that the results of this paper are in line with [S2], we further present the proof of Lemma in accordance with the proof in [S2] up to the fact that, following Assumption 2, in this paper the parameters $\beta$ are known, which allows one to avoid overparameterization in (11).

**Part I** (*parametrization of the regression equation* (11)). **Step 1.** The following error is considered:

$$\tilde{\xi}(t) = \xi(t) - z(t) - \Omega(t)\psi_a(\theta) - P(t)\psi_b(\theta). \tag{S1}$$

Then the derivative of (S1) is written:

$$\begin{gathered}\dot{\tilde{\xi}}(t) = A_0\xi(t) + \psi_a(\theta)y(t) + \psi_b(\theta)u(t) + \psi_d(\theta)\delta(t) - A_K z(t) - Ky(t) - (A_K\Omega(t) + I_n y(t))\psi_a(\theta) - \\ -(A_K P(t) + I_n u(t))\psi_b(\theta) = \\ = A_0\xi(t) - A_K z(t) - Ky(t) - A_K\Omega(t)\psi_a(\theta) - A_K P(t)\psi_b(\theta) + \psi_d(\theta)\delta(t) = A_K\tilde{\xi}(t) + \psi_d(\theta)\delta(t).\end{gathered} \tag{S2}$$

The solution of the differential equation (S2) is obtained:

$$\tilde{\xi}(t) = e^{A_K(t-t_0)}\tilde{\xi}(t_0) + \overline{\delta}(t), \tag{S3}$$

where the external disturbance $\overline{\delta}(t)$ is described by the following set of equations:

$$\begin{cases}\dot{\overline{\delta}}(t) = A_K\overline{\delta}(t) + \psi_d(\theta)\delta(t), \\ v_f(t) = C_0^{\mathrm{T}}\overline{\delta}(t).\end{cases} \tag{S4}$$

Having substituted (S3) into (S1), it is written:

$$\begin{gathered}e^{A_K(t-t_0)}\tilde{\xi}(t_0) + \overline{\delta}(t) = \xi(t) - z(t) - \Omega(t)\psi_a(\theta) - P(t)\psi_b(\theta) \\ \Updownarrow \\ \xi(t) = e^{A_K(t-t_0)}\tilde{\xi}(t_0) + \overline{\delta}(t) + z(t) + \Omega(t)\psi_a(\theta) + P(t)\psi_b(\theta).\end{gathered} \tag{S5}$$

Equation (S5) is multiplied by $C_0^{\mathrm{T}}$ to obtain:

$$y(t) = C_0^{\mathrm{T}}\xi(t) = C_0^{\mathrm{T}}z(t) + C_0^{\mathrm{T}}\Omega(t)\psi_a(\theta) + C_0^{\mathrm{T}}P(t)\psi_b(\theta) + v_f(t) + C_0^{\mathrm{T}}e^{A_K(t-t_0)}\tilde{\xi}(t_0). \tag{S6}$$

Owing to equation (S6), the function $\overline{q} = y(t) - C_0^{\mathrm{T}}z(t)$ is differentiated:

$$\dot{\overline{q}}(t) = C_0^{\mathrm{T}}\dot{\Omega}(t)\psi_a(\theta) + C_0^{\mathrm{T}}\dot{P}(t)\psi_b(\theta) + \dot{v}_f(t) + C_0^{\mathrm{T}}A_K e^{A_K(t-t_0)}\tilde{\xi}(t_0). \tag{S7}$$

**Step 2.** The aim is to parametrize the term $\dot{v}_f(t)$ of (S7) as a linear regression with measurable regressor. In order to achieve it, equation (S4) is rewritten as a transfer function:

$$v_f(t) = C_0^{\mathrm{T}}(sI_n - A_K)^{-1}\psi_d(\theta)\delta(t) = W_f[\delta(t)]. \tag{S8}$$

The derivative of the disturbance $\delta(t)$ is written as:

$$\dot{\delta}(t) = h_\delta^{\mathrm{T}}\mathcal{A}_\delta x_\delta(t) + \delta(t_0)D_\delta(t), \tag{S9}$$

where $D_\delta(t)$ is the Dirac function.

A virtual variable $\delta_d(t) = h_\delta^{\mathrm{T}}\mathcal{A}_\delta x_\delta(t)$ is introduced. Then the following equations hold:

$$\begin{gathered}\dot{x}_\delta(t) = \mathcal{A}_\delta x_\delta(t), \\ \delta_d(t) = \overline{h}_\delta^{\mathrm{T}}x_\delta(t),\ \overline{h}_\delta^{\mathrm{T}} = h_\delta^{\mathrm{T}}\mathcal{A}_\delta.\end{gathered} \tag{S10}$$

Equation (S8) is differentiated, and then (S9) and (S10) are substituted into the obtained result:

$$\dot{v}_f = sW_f[\delta(t)] = W_f\left[\dot{\delta}(t)\right] = W_f\left[h_\delta^{\mathrm{T}}A_\delta x_\delta(t) + \delta(t_0)D_\delta(t)\right] = \underbrace{W_f[\delta_d(t)]}_{v_f(t)} + W_f[\delta(t_0)D_\delta(t)]. \tag{S11}$$

Therefore, as $A_K$ is a Hurwitz matrix, it is enough to parametrize $v_f(t)$ to, in its turn, parametrize $\dot{v}_f(t)$. In order to achieve that, an auxiliary variable $\zeta(t) = M_\delta x_\delta(t)$ is introduced, where the matrix of linear similarity $M_\delta$ is the solution of the Sylvester equation:

$$M_\delta\mathcal{A}_\delta - GM_\delta = l\overline{h}_\delta^{\mathrm{T}}, \tag{S12}$$

which has a unique solution [S2] as, owing to Assumption 2, the pair $\left(h_\delta^{\mathrm{T}}, \mathcal{A}_\delta\right)$ is observable and, following the premises of Lemma 1, the pair $(G, l)$ is controllable and $\sigma\{\mathcal{A}_\delta\} \cap \sigma\{G\} = 0$.

Having differentiated $\zeta(t)$, it is obtained:

$$\dot{\zeta}(t) = M_\delta\mathcal{A}_\delta x_\delta(t) = GM_\delta x_\delta(t) + l\overline{h}_\delta^{\mathrm{T}}x_\delta(t) = G\zeta(t) + l\delta_d(t), \tag{S13}$$

from which, owing to $x_\delta(t) = M_\delta^{-1}\zeta(t)$, it follows that:

$$\delta_d(t) = \overline{h}_\delta^{\mathrm{T}} M_\delta^{-1}\zeta = \beta^{\mathrm{T}}\zeta,\ \beta = \overline{h}_\delta^{\mathrm{T}} M_\delta^{-1}. \tag{S14}$$

Considering (S14), equation (S11) is rewritten as:

$$\dot{\upsilon}_f = W_f\left[\beta^{\mathrm{T}}\zeta(t)\right] + W_f\left[\delta(t_0)D_\delta(t)\right] = \beta^{\mathrm{T}}W_f\left[\zeta(t)\right] + W_f\left[\delta(t_0)D_\delta(t)\right] = \beta^{\mathrm{T}}\zeta_w(t) + W_f\left[\delta(t_0)D_\delta(t)\right]. \tag{S15}$$

Instead of $\delta_d(t)$, the filter (S13) is applied to the signal $\upsilon_f(t)$:

$$\zeta_f(t) = (sI - G)^{-1} l\left[\upsilon_f(t)\right] + e^{G(t-t_0)}\zeta_f(t_0), \tag{S16}$$

then, with $\zeta(t) = (sI - G)^{-1} l\left[\delta_d(t)\right] + e^{G(t-t_0)}\zeta(t_0)$ in mind, it is obtained:

$$\begin{gathered}\zeta_w(t) = W_f\left[\zeta(t)\right] = W_f\left[(sI - G)^{-1} l\left[\delta_d(t)\right] + e^{G(t-t_0)}\zeta(t_0)\right] = (sI-G)^{-1} l W_f\left[\delta_d(t)\right] + W_f\left[e^{G(t-t_0)}\zeta(t_0)\right] = \\ = (sI-G)^{-1} l \upsilon_f + W_f\left[e^{G(t-t_0)}\zeta(t_0)\right] = \zeta_f(t) - e^{G(t-t_0)}\zeta_f(t_0) + W_f\left[e^{G(t-t_0)}\zeta(t_0)\right].\end{gathered} \tag{S17}$$

Equation (S17) is substituted into (S15) to obtain:

$$\dot{\upsilon}_f(t) = \beta^{\mathrm{T}}\zeta_f(t) - \beta^{\mathrm{T}}e^{G(t-t_0)}\zeta_f(t_0) + \beta^{\mathrm{T}}W_f\left[e^{G(t-t_0)}\xi(t_0)\right] + W_f\left[\delta(t_0)D_\delta(t)\right]. \tag{S18}$$

The observer $\zeta_f(t)$ is introduced in the following form:

$$\hat{\zeta}_f(t) = F(t) + H(t)\psi_b(\theta) + N(t)\psi_a(\theta) + ly(t). \tag{S19}$$

The error $\tilde{\zeta}_f(t) = \zeta_f(t) - \hat{\zeta}_f(t)$ is differentiated using (S7), (S11), (S16), (S19) to obtain:

$$\begin{gathered}\dot{\tilde{\zeta}}_f = G\zeta_f(t) + l\upsilon_f(t) - GF(t) - Gly(t) + lC_0^{\mathrm{T}}\dot{z}(t) - \left(GH(t) - lC_0^{\mathrm{T}}\dot{P}(t)\right)\psi_b(\theta) - \left(GN(t) - lC_0^{\mathrm{T}}\dot{\Omega}(t)\right)\psi_a(\theta) - \\ -lC_0^{\mathrm{T}}\dot{z}(t) - lC_0^{\mathrm{T}}\dot{\Omega}(t)\psi_a(\theta) - lC_0^{\mathrm{T}}\dot{P}(t)\psi_b(\theta) - l\left(\upsilon_f(t) + W_f\left[\delta(t_0)D_\delta(t)\right]\right) - lC_0^{\mathrm{T}}A_K e^{A_K(t-t_0)}\tilde{\xi}(t_0) = \\ = G\zeta_f(t) - \underbrace{GF(t) - Gly(t) - GH(t)\psi_b(\theta) - GN(t)\psi_a(\theta)}_{G\hat{\zeta}_f(t)} - lW_f\left[\delta(t_0)D_\delta(t)\right] - lC_0^{\mathrm{T}}A_K e^{A_K(t-t_0)}\tilde{\xi}(t_0) = \\ = G\tilde{\zeta}_f - lC_0^{\mathrm{T}}A_K e^{A_K(t-t_0)}\tilde{\xi}(t_0) - lW_f\left[\delta(t_0)D_\delta(t)\right].\end{gathered} \tag{S20}$$

The solution of equation (S20) is written as:

$$\tilde{\zeta}_f(t) = \zeta_f(t) - \hat{\zeta}_f(t) = e^{G(t-t_0)}\tilde{\zeta}_f(t_0) - \mathfrak{H}\left[C_0^{\mathrm{T}}A_K e^{A_K(t-t_0)}\tilde{\xi}(t_0) + W_f\left[\delta(t_0)D_\delta(t)\right]\right], \tag{S21}$$

so (S18) is rewritten as:

$$\begin{gathered}\dot{\upsilon}_f(t) = \beta^{\mathrm{T}}\hat{\zeta}_f(t) + \beta^{\mathrm{T}}e^{G(t-t_0)}\tilde{\zeta}_f(t_0) - \beta^{\mathrm{T}}\mathfrak{H}\left[C_0^{\mathrm{T}}A_K e^{A_K(t-t_0)}\tilde{\xi}(t_0) + W_f\left[\delta(t_0)D_\delta(t)\right]\right] - \\ -\beta^{\mathrm{T}}e^{G(t-t_0)}\zeta_f(t_0) + \beta^{\mathrm{T}}W_f\left[e^{G(t-t_0)}\xi(t_0)\right] + W_f\left[\delta(t_0)D_\delta(t)\right] = \\ = \beta^{\mathrm{T}}\left(F(t) + ly(t)\right) + \beta^{\mathrm{T}}H(t)\psi_b(\theta) + \beta^{\mathrm{T}}N(t)\psi_a(\theta) + \\ +\beta^{\mathrm{T}}e^{G(t-t_0)}\tilde{\zeta}_f(t_0) - \beta^{\mathrm{T}}\mathfrak{H}\left[C_0^{\mathrm{T}}A_K e^{A_K(t-t_0)}\tilde{\xi}(t_0) + W_f\left[\delta(t_0)D_\delta(t)\right]\right] - \\ -\beta^{\mathrm{T}}e^{G(t-t_0)}\zeta_f(t_0) + \beta^{\mathrm{T}}W_f\left[e^{G(t-t_0)}\xi(t_0)\right] + W_f\left[\delta(t_0)D_\delta(t)\right],\end{gathered} \tag{S22}$$

where $\mathfrak{H}[.] = (sI-G)^{-1} l[.]$.

Equation (S22) is substituted into (S7) to obtain:

$$\begin{gathered}\dot{\overline{q}} = C_0^{\mathrm{T}}\dot{\Omega}(t)\psi_a(\theta) + C_0^{\mathrm{T}}\dot{P}(t)\psi_b(\theta) + \beta^{\mathrm{T}}\left(F(t) + ly(t)\right) + \beta^{\mathrm{T}}H(t)\psi_b(\theta) + \beta^{\mathrm{T}}N(t)\psi_a(\theta) + \\ +\beta^{\mathrm{T}}e^{G(t-t_0)}\tilde{\zeta}_f(t_0) - \beta^{\mathrm{T}}\mathfrak{H}\left[C_0^{\mathrm{T}}A_K e^{A_K(t-t_0)}\tilde{\xi}(t_0) + W_f\left[\delta(t_0)D_\delta(t)\right]\right] - \\ -\beta^{\mathrm{T}}e^{G(t-t_0)}\zeta_f(t_0) + \beta^{\mathrm{T}}W_f\left[e^{G(t-t_0)}\xi(t_0)\right] + W_f\left[\delta(t_0)D_\delta(t)\right] + C_0^{\mathrm{T}}A_K e^{A_K(t-t_0)}\tilde{\xi}(t_0) = \\ = \overline{\varphi}^{\mathrm{T}}(t)\eta(\theta) + \beta^{\mathrm{T}}\left(F(t) + ly(t)\right) + \overline{\varepsilon}(t),\end{gathered} \tag{S23}$$

where $\overline{\varepsilon}(t)$ denotes the sum of the exponentially decaying functions.

**Step 3.** The aim is to transform (S23) into (11) using the dynamic regressor extension and mixing method. In order to achieve it, the equation $\chi(t) = \overline{q}(t) - k_1\overline{q}_f(t)$ is differentiated using (S23), (14) to obtain:

$$\begin{gathered}\dot{\chi}(t) = \overline{\varphi}^{\mathrm{T}}(t)\eta(\theta) + \beta^{\mathrm{T}}\left(F(t) + ly(t)\right) + \overline{\varepsilon}(t) - k_1\left(-k_1\overline{q}_f(t) + \overline{q}(t)\right) = \\ = -k_1\chi(t) + \overline{\varphi}^{\mathrm{T}}(t)\eta(\theta) + \beta^{\mathrm{T}}\left(F(t) + ly(t)\right) + \overline{\varepsilon}(t).\end{gathered} \tag{S24}$$

The solution of (S24) allows one to obtain:

$$\overline{q}(t) - k_1\overline{q}_f(t) - \beta^{\mathrm{T}}(F_f(t) + l y_f(t)) = e^{-k_1(t-t_0)}\overline{q}(t_0) + \overline{\varphi}_f^{\mathrm{T}}(t)\,\eta(\theta) + \overline{\varepsilon}_f(t), \tag{S25}$$

where $\dot{\overline{\varepsilon}}_f(t) = -k_1\overline{\varepsilon}_f(t) + k_1\overline{\varepsilon}(t),\, \overline{\varepsilon}_f(t_0) = 0.$.

Using (S25), the first equation from (13) is written as:

$$q(t) = \varphi(t)\,\eta(\theta) + \varepsilon(t), \tag{S26}$$

where $\varepsilon(t) = \int\limits_{t_\epsilon}^{t} e^{-\sigma(\tau - t_\epsilon)}\overline{\varphi}_f(\tau)\left(\overline{\varepsilon}_f(t) + e^{-k_1(t-t_0)}\overline{q}(t_0)\right)d\tau,\, \varepsilon(t_\epsilon) = 0_{2n}$.

The disturbance $\overline{\varepsilon}_f(t) + e^{-k_1(\tau - t_0)}\overline{q}(t_0)$ vanishes exponentially for all $t \geqslant t_0$, thus, if $t_\epsilon \gg t_0$, then (S26) is rewritten as:

$$q(t) = \varphi(t)\,\eta(\theta) + o(\varphi(t)\,\eta(\theta)), \tag{S27}$$

so the contribution of $\varepsilon(t)$ into the function $q(t)$ is negligible, and, if $t_\epsilon$ is chosen to be sufficiently large, then $q(t) := \varphi(t)\,\eta(\theta)$. Having multiplied $q(t)$ by $k(t)\cdot\mathrm{adj}\{\varphi(t)\}$ and applied $\mathrm{adj}\{\varphi(t)\}\,\varphi(t) = \det\{\varphi(t)\}\,I_{2n}$, equation (11) is obtained.

As signals $y(t),\, u(t)$ are bounded according to Assumption 1, then, owing to the stability of the filters (14), (15) and exponential decay of integrands from (13), for all $t \geqslant t_0$ the inequality $\Delta_{\max} \geqslant \Delta(t)$ holds. According to Lemma 6.8 from [S3], if $\overline{\varphi}(t) \in \mathrm{FE}$, then it also holds that $\overline{\varphi}_f(t) \in \mathrm{FE}$. Using the results of Theorem 1 from [S4], if $\overline{\varphi}_f(t) \in \mathrm{FE}$, then for all $t \geqslant t_e$ it holds that $\varphi(t) > 0 \Leftrightarrow \Delta(t) \geqslant \Delta_{\min} > 0$, which completes the proof of the fact that equation (11) can be obtained using the proposed parametrization.

**Part II** (*regression equation (12) parametrization*). The following error is considered:

$$\tilde{\xi}(t) = \xi(t) - z(t) - R^{\mathrm{T}}(t)\,\kappa(\theta) = \xi(t) - z(t) - \Omega(t)\,\psi_a(\theta) - P(t)\,\psi_b(\theta) - U(t)\,\psi_d(\theta). \tag{S28}$$

The derivative of (S28) is written as:

$$\begin{gathered}\dot{\tilde{\xi}}(t) = A_0\xi(t) + \psi_a(\theta)\,y(t) + \psi_b(\theta)\,u(t) + \psi_d(\theta)\,\delta(t) - A_K z(t) - Ky(t) - (A_K\Omega(t) + I_n y(t))\,\psi_a(\theta) - \\ - (A_K P(t) + I_n u(t))\,\psi_b(\theta) - (A_K U(t) + I_n\delta(t))\,\psi_d(\theta) = \\ = A_0\xi(t) - A_K z(t) - Ky(t) - A_K\Omega(t)\,\psi_a(\theta) - A_K P(t)\,\psi_b(\theta) - A_K U(t)\,\psi_d(\theta) = \\ = A_K\tilde{\xi}(t).\end{gathered} \tag{S29}$$

The solution of the differential equation (S29) takes the following form:

$$\tilde{\xi}(t) = e^{A_K(t-t_0)}\tilde{\xi}(t_0), \tag{S30}$$

which, in accordance with (S28), means that, if $t_\epsilon \gg t_0$, then the inequality (12) holds, as was to be proved. ■

## II. Proof of Lemma 2 in the Manuscript

***Lemma 2.*** *The unknown parameters $\kappa(\theta)$, $T_I(\theta)$ and $x_{\delta 0}$ for all $t \geq t_\epsilon$ satisfy measurable regression equations:*

$$\begin{gathered}\mathcal{Y}_\kappa(t) = \mathcal{M}_\kappa(t)\,\kappa(\theta), \\ \mathcal{Y}_\kappa(t) = \mathrm{adj}\{\mathrm{blkdiag}\{\Delta(t)\,I_{2n},\, \mathcal{M}_{\psi_d}(t)\,I_n\}\}\begin{bmatrix}\mathcal{Y}(t) \\ \mathcal{Y}_{\psi_d}(t)\end{bmatrix}, \\ \mathcal{M}_\kappa(t) = \det\{\mathrm{blkdiag}\{\Delta(t)\,I_{2n},\, \mathcal{M}_{\psi_d}(t)\,I_n\}\},\end{gathered}$$

$$\begin{gathered}\mathcal{Y}_{T_I}(t) = \mathcal{M}_{T_I}(t)\,T_I(\theta), \\ \mathcal{Y}_{T_I}(t) = \mathrm{adj}\left\{\mathcal{T}_\mathcal{P}\left(\Xi_\mathcal{P}(\mathcal{M}_\theta)\,\mathcal{Y}_\theta\right)\right\}\mathcal{T}_\mathcal{Q}\left(\Xi_\mathcal{Q}(\mathcal{M}_\theta)\,\mathcal{Y}_\theta\right), \\ \mathcal{M}_{T_I}(t) = \det\left\{\mathcal{T}_\mathcal{P}\left(\Xi_\mathcal{P}(\mathcal{M}_\theta)\,\mathcal{Y}_\theta\right)\right\},\end{gathered}$$

$$\begin{gathered}\mathcal{Y}_{x_{\delta 0}}(t) = \mathcal{M}_{x_{\delta 0}}(t)\,x_{\delta 0}, \\ \mathcal{Y}_{x_{\delta 0}}(t) = \mathrm{adj}\{V_f(t)\}\,p_f(t),\, \mathcal{M}_{x_{\delta 0}}(t) = \det\{V_f(t)\},\end{gathered}$$

*where*

1) *the regression $\mathcal{Y}_\theta(t) = \mathcal{M}_\theta(t)\,\theta$ is formed using the following equations:*

$$\begin{gathered}\mathcal{Y}_\theta(t) = \mathrm{adj}\left\{\mathcal{T}_\mathcal{G}\left(\Xi_\mathcal{G}(\Delta)\,\mathcal{Y}_{ab}\right)\right\}\mathcal{T}_\mathcal{S}\left(\Xi_\mathcal{S}(\Delta)\,\mathcal{Y}_{ab}\right), \\ \mathcal{M}_\theta(t) = \det\left\{\mathcal{T}_\mathcal{G}\left(\Xi_\mathcal{G}(\Delta)\,\mathcal{Y}_{ab}\right)\right\},\, \mathcal{Y}_{ab}(t) = \mathcal{L}_{ab}\mathcal{Y}(t),\end{gathered}$$

2) *the regression* $\mathcal{Y}_{\psi_d}(t)=\mathcal{M}_{\psi_d}(t)\,\psi_d(\theta)$ *is formed using the following equations:*

$$\begin{gathered}\mathcal{Y}_{\psi_d}(t)=\operatorname{adj}\left\{\mathcal{T}_{\mathcal{R}}\left(\Xi_{\mathcal{R}}\left(\mathcal{M}_\theta\right)\mathcal{Y}_\theta\right)\right\}\mathcal{T}_{\mathcal{W}}\left(\Xi_{\mathcal{W}}\left(\mathcal{M}_\theta\right)\mathcal{Y}_\theta\right),\\ \mathcal{M}_{\psi_d}(t)=\det\left\{\mathcal{T}_{\mathcal{R}}\left(\Xi_{\mathcal{R}}\left(\mathcal{M}_\theta\right)\mathcal{Y}_\theta\right)\right\},\end{gathered}$$

3) *the signals* $p_f(t)$ *and* $V_f(t)$ *are obtained as follows:*

$$\begin{gathered}p_f(t)=\int\limits_{t_\epsilon}^{t}e^{-\sigma(\tau-t_\epsilon)}\Delta(\tau)\left(I_{n_\delta}\otimes\mathcal{Y}_{\psi_d}(\tau)\right)^{\mathrm{T}}V^{\mathrm{T}}(\tau)\,C_0\mathcal{M}_{\psi_d}(\tau)\,p(\tau)\,d\tau,\;\;p_f(t_\epsilon)=0_{n_\delta},\\ p(t)=\Delta(t)\,\overline{q}(t)-C_0^{\mathrm{T}}\Omega(t)\,\mathcal{L}_a\mathcal{Y}(t)-C_0^{\mathrm{T}}P(t)\,\mathcal{L}_b\mathcal{Y}(t),\\ \mathcal{L}_a\psi_{ab}(\theta)=\psi_a(\theta),\,\mathcal{L}_b\psi_{ab}(\theta)=\psi_b(\theta),\\ V_f(t)=\int\limits_{t_\epsilon}^{t}e^{-\sigma(\tau-t_\epsilon)}\Delta^2(\tau)\left(I_{n_\delta}\otimes\mathcal{Y}_{\psi_d}(\tau)\right)^{\mathrm{T}}V^{\mathrm{T}}(\tau)\,C_0C_0^{\mathrm{T}}V(\tau)\left(I_{n_\delta}\otimes\mathcal{Y}_{\psi_d}(\tau)\right)d\tau,\;\;V_f(t_\epsilon)=0_{n_\delta\times n_\delta},\\ \dot{V}(t)=A_KV(t)+\left(h_\delta^{\mathrm{T}}\Phi_\delta(t)\otimes I_n\right),\,V(t_0)=0_{n\times nn_\delta},\end{gathered}$$

*and, if* $\overline{\varphi}(t)\in\mathrm{FE}$ *and* $\left(h_\delta^{\mathrm{T}}\Phi_\delta(t)\otimes I_n\right)\in\mathrm{FE}$ *over* $[t_\epsilon;\,t_e]$*, then for all* $t\geq t_e$ *it holds that:*

$$\begin{gathered}\left|\mathcal{M}_\kappa(t)\right|\geq\underline{\mathcal{M}_\kappa}>0,\;\left|\mathcal{M}_{T_I}(t)\right|\geq\underline{\mathcal{M}_{T_I}}>0,\\ \left|\mathcal{M}_{x_{\delta0}}(t)\right|\geq\underline{\mathcal{M}_{x_{\delta0}}}>0.\end{gathered}$$

*Proof:* According to Definition 1 and (17) and owing to:

$$\begin{gathered}\Xi_{\mathcal{S}}(\Delta(t))=\overline{\Xi}_{\mathcal{S}}(\Delta(t))\,\Delta(t),\,\Xi_{\mathcal{G}}(\Delta(t))=\overline{\Xi}_{\mathcal{G}}(\Delta(t))\,\Delta(t),\\ \mathcal{Y}_{ab}(t)=\mathcal{L}_{ab}\mathcal{Y}(t)=\Delta(t)\,\mathcal{L}_{ab}\eta(\theta)=\Delta(t)\,\psi_{ab}(\theta),\\ \overline{\Xi}_{\mathcal{S}}(\Delta(t))\,\Delta(t)\,\psi_{ab}(\theta)=\overline{\Xi}_{\mathcal{S}}(\Delta(t))\,\mathcal{Y}_{ab}(t),\\ \overline{\Xi}_{\mathcal{G}}(\Delta(t))\,\Delta(t)\,\psi_{ab}(\theta)=\overline{\Xi}_{\mathcal{G}}(\Delta(t))\,\mathcal{Y}_{ab}(t),\end{gathered}$$

it follows from (11) that:

$$\mathcal{T}_{\mathcal{S}}\left(\overline{\Xi}_{\mathcal{S}}(\Delta(t))\,\mathcal{Y}_{ab}(t)\right)=\mathcal{T}_{\mathcal{G}}\left(\overline{\Xi}_{\mathcal{G}}(\Delta(t))\,\mathcal{Y}_{ab}(t)\right)\theta.\tag{S31}$$

Then, having multiplied (S31) by $\operatorname{adj}\left\{\mathcal{T}_{\mathcal{G}}\left(\overline{\Xi}_{\mathcal{G}}(\Delta(t))\,\mathcal{Y}_{ab}(t)\right)\right\}$, the following regression equation is obtained:

$$\mathcal{Y}_\theta(t)=\mathcal{M}_\theta(t)\,\theta,\tag{S32}$$

using which together with (18), (19) and:

$$\Xi_{(.)}\left(\mathcal{M}_\theta(t)\right)=\overline{\Xi}_{(.)}\left(\mathcal{M}_\theta(t)\right)\mathcal{M}_\theta(t),$$

it is obtained that:

$$\mathcal{T}_{\mathcal{Q}}\left(\overline{\Xi}_{\mathcal{Q}}\left(\mathcal{M}_\theta(t)\right)\mathcal{Y}_\theta(t)\right)=\mathcal{T}_{\mathcal{P}}\left(\overline{\Xi}_{\mathcal{P}}\left(\mathcal{M}_\theta(t)\right)\mathcal{Y}_\theta(t)\right)T_I(\theta),\tag{S33}$$

$$\mathcal{T}_{\mathcal{W}}\left(\overline{\Xi}_{\mathcal{W}}\left(\mathcal{M}_\theta(t)\right)\mathcal{Y}_\theta(t)\right)=\mathcal{T}_{\mathcal{R}}\left(\overline{\Xi}_{\mathcal{R}}\left(\mathcal{M}_\theta(t)\right)\mathcal{Y}_\theta(t)\right)\psi_d(\theta).\tag{S34}$$

Equation (S33) is multiplied by $\operatorname{adj}\left\{\mathcal{T}_{\mathcal{P}}\left(\overline{\Xi}_{\mathcal{P}}\left(\mathcal{M}_\theta(t)\right)\mathcal{Y}_\theta(t)\right)\right\}$ to obtain $\mathcal{Y}_{T_I}(t)=\mathcal{M}_{T_I}(t)\,T_I(\theta)$ and, as a result, equation (21).

Equation (S34) is multiplied by $\operatorname{adj}\left\{\mathcal{T}_{\mathcal{R}}\left(\overline{\Xi}_{\mathcal{R}}\left(\mathcal{M}_\theta(t)\right)\mathcal{Y}_\theta(t)\right)\right\}$ to obtain $\mathcal{Y}_{\psi_d}(t)=\mathcal{M}_{\psi_d}(t)\,\psi_d(\theta)$ and, as a result, equation (20).

The next aim is to derive the regression equation w.r.t. $x_{\delta0}$. Using the properties of the vectorization operation:

$$\begin{gathered}vec\left(\psi_d(\theta)\,h_\delta^{\mathrm{T}}\Phi_\delta(t)\,x_{\delta0}\right)=\underbrace{\left(x_{\delta0}^{\mathrm{T}}\otimes\psi_d(\theta)\right)}_{n\times n_\delta}\underbrace{vec\left(h_\delta^{\mathrm{T}}\Phi_\delta\right)}_{n_\delta},\\ vec\left(\left(x_{\delta0}^{\mathrm{T}}\otimes\psi_d(\theta)\right)vec\left(h_\delta^{\mathrm{T}}\Phi_\delta(t)\right)\right)=\underbrace{\left(h_\delta^{\mathrm{T}}\Phi_\delta(t)\otimes I_n\right)}_{n\times nn_\delta}\underbrace{vec\left(x_{\delta0}^{\mathrm{T}}\otimes\psi_d(\theta)\right)}_{nn_\delta},\end{gathered}$$

equation (6) is rewritten as:

$$\dot{\xi}(t)=A_0\xi(t)+\psi_a(\theta)\,y(t)+\psi_b(\theta)\,u(t)+\left(h_\delta^{\mathrm{T}}\Phi_\delta(t)\otimes I_n\right)vec\left(x_{\delta0}^{\mathrm{T}}\otimes\psi_d(\theta)\right).\tag{S35}$$

The following error is introduced:

$$e(t)=\xi(t)-z(t)-\Omega(t)\,\psi_a(\theta)-P(t)\,\psi_b(\theta)-V(t)\,vec\left(x_{\delta0}^{\mathrm{T}}\otimes\psi_d(\theta)\right).\tag{S36}$$

Equation (S36) is differentiated and, similarly to (S29), we obtain $\dot{e}(t)=A_Ke(t)$. Then (S36) is multiplied by $C_0^{\mathrm{T}}$ to have:

$$\overline{q}(t)=C_0^{\mathrm{T}}e^{A_K(t-t_0)}e(t_0)+C_0^{\mathrm{T}}\Omega(t)\,\psi_a(\theta)+C_0^{\mathrm{T}}P(t)\,\psi_b(\theta)+C_0^{\mathrm{T}}V(t)\,vec\left(x_{\delta0}^{\mathrm{T}}\otimes\psi_d(\theta)\right).\tag{S37}$$

Using the following properties:

$$x_{\delta 0}^{\mathrm{T}} \otimes \psi_d(\theta) = \psi_d(\theta)\, x_{\delta 0}^{\mathrm{T}},$$
$$vec\left(\psi_d(\theta)\, x_{\delta 0}^{\mathrm{T}}\right) = \underbrace{\left(I_{n_\delta} \otimes \psi_d(\theta)\right)}_{nn_\delta \times n_\delta} x_{\delta 0},$$

equation (S37) is rewritten as:

$$\overline{q}(t) = C_0^{\mathrm{T}} e^{A_K(t-t_0)} e(t_0) + C_0^{\mathrm{T}} \Omega(t)\, \psi_a(\theta) + C_0^{\mathrm{T}} P(t)\, \psi_b(\theta) + C_0^{\mathrm{T}} V(t) \left(I_{n_\delta} \otimes \psi_d(\theta)\right) x_{\delta 0}. \tag{S38}$$

The following auxiliary signal is introduced to cancel out the effect of the terms $C_0^{\mathrm{T}} \Omega(t)\, \psi_a(\theta) + C_0^{\mathrm{T}} P(t)\, \psi_b(\theta)$:

$$\overline{p}_e = \Delta(t)\, C_0^{\mathrm{T}} \Omega(t)\, \psi_a(\theta) + \Delta(t)\, C_0^{\mathrm{T}} P(t)\, \psi_b(\theta) = C_0^{\mathrm{T}} \Omega(t)\, \mathcal{L}_a \mathcal{Y}(t) + C_0^{\mathrm{T}} P(t)\, \mathcal{L}_b \mathcal{Y}(t)\,. \tag{S39}$$

Equation (S38) is multiplied by $\Delta(t)$, and (S39) is subtracted from the obtained result to have:

$$\begin{gathered} p(t) = \Delta(t)\, \overline{q}(t) - \overline{p}_e(t) = \Delta(t)\, C_0^{\mathrm{T}} V(t) \left(I_{n_\delta} \otimes \psi_d(\theta)\right) x_{\delta 0} + \Delta(t)\, C_0^{\mathrm{T}} e^{A_K(t-t_0)} e(t_0) = \\ = \Delta(t)\, C_0^{\mathrm{T}} V(t) \left(I_{n_\delta} \otimes \psi_d(\theta)\right) x_{\delta 0} + \Delta(t)\, C_0^{\mathrm{T}} e^{A_K(t-t_0)} e(t_0)\,. \end{gathered} \tag{S40}$$

Equation (S40) is multiplied by $\mathcal{M}_{\psi_d}(t)$, and $\mathcal{Y}_{\psi_d}(t) = \mathcal{M}_{\psi_d}(t)\, \psi_d(\theta)$ is substituted into the obtained result to have:

$$\begin{gathered} \mathcal{M}_{\psi_d}(t)\, p(t) = \mathcal{M}_{\psi_d}(t)\, \Delta(t)\, C_0^{\mathrm{T}} V(t) \left(I_{n_\delta} \otimes \psi_d(\theta)\right) x_{\delta 0} = \\ = \Delta(t)\, C_0^{\mathrm{T}} V(t) \left(I_{n_\delta} \otimes \mathcal{Y}_{\psi_d}(t)\right) x_{\delta 0} + \mathcal{M}_{\psi_d}(t)\, \Delta(t)\, C_0^{\mathrm{T}} e^{A_K(t-t_0)} e(t_0)\,. \end{gathered}$$

The term $\mathcal{M}_{\psi_d}(t)\, \Delta(t)\, C_0^{\mathrm{T}} e^{A_K(t-t_0)} e(t_0)$ exponentially vanishes for all $t \geqslant t_0$, thus, if $t_\epsilon \gg t_0$, then its contribution is negligible, and for all $t \geqslant t_\epsilon$ the above-given equation is rewritten as:

$$\begin{gathered} \mathcal{M}_{\psi_d}(t)\, p(t) = \Delta(t)\, C_0^{\mathrm{T}} V(t) \left(I_{n_\delta} \otimes \mathcal{Y}_{\psi_d}(t)\right) x_{\delta 0} + o\left(\Delta(t)\, C_0^{\mathrm{T}} V(t) \left(I_{n_\delta} \otimes \mathcal{Y}_{\psi_d}(t)\right) x_{\delta 0}\right) = \\ = \Delta(t)\, C_0^{\mathrm{T}} V(t) \left(I_{n_\delta} \otimes \mathcal{Y}_{\psi_d}(t)\right) x_{\delta 0}. \end{gathered} \tag{S41}$$

Equation (S41) is filtered using (24), and the obtained result is multiplied by $\operatorname{adj}\{V_f(t)\}$ to have $\mathcal{Y}_{x_{\delta 0}}(t) = \mathcal{M}_{x_{\delta 0}}(t)\, x_{\delta 0}$ and, in its turn, equation (22).

Using the results from Lemma 1, if $\overline{\varphi}(t) \in \mathrm{FE}$, then for all $t \geqslant t_e$ it holds that $\Delta(t) \geqslant \Delta_{\min} > 0$, and, following hypotheses (17)-(19), we have:

$$\begin{gathered} \det{}^2\{\mathcal{G}(\psi_{ab})\} > 0,\ \det{}^2\{\mathcal{P}(\theta)\} > 0,\ \det{}^2\{\mathcal{R}(\theta)\} > 0, \\ \det\{\Pi_\theta(\Delta(t))\} \geqslant \Delta^{\ell_\Theta}(t)\,,\ \det\{\Pi_{T_I}(\mathcal{M}_\theta(t))\} \geqslant \mathcal{M}_\theta^{\ell_{T_I}}(t)\,,\ \det\{\Pi_{\psi_d}(\mathcal{M}_\theta(t))\} \geqslant \mathcal{M}_\theta^{\ell_{\psi_d}}(t)\,, \end{gathered}$$

from which it is concluded that, if $\overline{\varphi}(t) \in \mathrm{FE}$, then for all $t \geqslant t_e$ it holds that:

$$\begin{gathered} |\mathcal{M}_\theta(t)| = |\det\{\mathcal{T}_\mathcal{G}(\Xi_\mathcal{G}(\Delta(t))\, \psi_{ab})\}| = |\det\{\Pi_\theta(\Delta(t))\} \det\{\mathcal{G}(\psi_{ab})\}| \geqslant \\ \geqslant |\det\{\mathcal{G}(\psi_{ab})\}|\, \Delta_{\min}^{\ell_\theta} = \underline{\mathcal{M}_\theta} > 0, \\ |\mathcal{M}_{\psi_d}(t)| = |\det\{\mathcal{T}_\mathcal{R}(\Xi_\mathcal{R}(\mathcal{M}_\theta(t))\, \theta)\}| = |\det\{\mathcal{R}(\theta)\} \det\{\Pi_{\psi_d}(\mathcal{M}_\theta(t))\}| \geqslant \\ \geqslant |\det\{\mathcal{R}(\theta)\}| \left|\mathcal{M}_\theta^{\psi_d}(t)\right| \geqslant |\det\{\mathcal{R}(\theta)\}| \left|\det{}^{\psi_d}\{\mathcal{G}(\psi_{ab})\}\right| \Delta_{\min}^{\ell_\theta \psi_d} = \underline{\mathcal{M}_{\psi_d}} > 0, \\ |\mathcal{M}_\kappa(t)| = \left|\Delta^{2n}(t)\, \mathcal{M}_{\psi_d}^n(t)\right| \geqslant \Delta_{\min}^{2n} \underline{\mathcal{M}_{\psi_d}^n} > 0, \\ |\mathcal{M}_{T_I}(t)| = |\det\{\mathcal{T}_\mathcal{P}(\Xi_\mathcal{P}(\mathcal{M}_\theta(t))\, \theta)\}| = |\det\{\mathcal{P}(\theta)\} \det\{\Pi_{T_I}(\mathcal{M}_\theta(t))\}| \geqslant \\ \geqslant |\det\{\mathcal{P}(\theta)\}| \left|\mathcal{M}_\theta^{T_I}(t)\right| \geqslant |\det\{\mathcal{P}(\theta)\}| \left|\det{}^{T_I}\{\mathcal{G}(\psi_{ab})\}\right| \Delta_{\min}^{\ell_\theta T_I} = \underline{\mathcal{M}_{T_I}} > 0. \end{gathered} \tag{S42}$$

To obtain the low bound of the regressor $\mathcal{M}_{x_{\delta 0}}(t)$, first of all, the low bound of $V_f(t)$ is written when $\overline{\varphi}(t) \in \mathrm{FE}$ and $\left(h_\delta^{\mathrm{T}} \Phi_\delta(t) \otimes I_n\right) \in \mathrm{FE}$:

$$
\begin{aligned}
&V_f(t) = \int_{t_\epsilon}^{t} e^{-\sigma(\tau - t_\epsilon)} \Delta^2(\tau) \left(I_{n_\delta} \otimes \mathcal{Y}_{\psi_d}(\tau)\right)^{\mathrm{T}} V^{\mathrm{T}}(\tau) C_0 C_0^{\mathrm{T}} V(\tau) \left(I_{n_\delta} \otimes \mathcal{Y}_{\psi_d}(\tau)\right) d\tau = \\
&= \left(I_{n_\delta} \otimes \psi_d(\theta)\right)^{\mathrm{T}} \int_{t_\epsilon}^{t} e^{-\sigma(\tau - t_\epsilon)} \mathcal{M}_{\psi_d}^2(\tau) \Delta^2(\tau) V^{\mathrm{T}}(\tau) C_0 C_0^{\mathrm{T}} V(\tau) d\tau \left(I_{n_\delta} \otimes \psi_d(\theta)\right) \geqslant \\
&\geqslant \underline{\mathcal{M}_{\psi_d}^2} \Delta_{\min}^2 \left(I_{n_\delta} \otimes \psi_d(\theta)\right)^{\mathrm{T}} \int_{t_\epsilon}^{t} e^{-\sigma(\tau - t_\epsilon)} V^{\mathrm{T}}(\tau) C_0 C_0^{\mathrm{T}} V(\tau) d\tau \left(I_{n_\delta} \otimes \psi_d(\theta)\right) \geqslant \\
&\geqslant \underline{\mathcal{M}_{\psi_d}^2} \Delta_{\min}^2 \left(I_{n_\delta} \otimes \psi_d(\theta)\right)^{\mathrm{T}} e^{-\sigma(t_e - t_\epsilon)} \int_{t_\epsilon}^{t_e} V^{\mathrm{T}}(\tau) C_0 C_0^{\mathrm{T}} V(\tau) d\tau \left(I_{n_\delta} \otimes \psi_d(\theta)\right).
\end{aligned} \tag{S43}
$$

In accordance with Lemma 6.8. from [S3], if $\left(h_\delta^{\mathrm{T}} \Phi_\delta(t) \otimes I_n\right) \in \mathrm{FE}$, then the following inequality holds over $[t_\epsilon; t_e]$:

$$
\int_{t_\epsilon}^{t_e} V^{\mathrm{T}}(\tau) C_0 C_0^{\mathrm{T}} V(\tau) d\tau \geqslant \alpha I_{n n_\delta}, \tag{S44}
$$

and using the properties of the Kronecker product, it is obtained that:

$$
\left(I_{n_\delta} \otimes \psi_d(\theta)\right)^{\mathrm{T}} \underbrace{\left(I_{n_\delta} \otimes \psi_d(\theta)\right)}_{n n_\delta \times n_\delta} = \left(I_{n_\delta}^{\mathrm{T}} \otimes \psi_d^{\mathrm{T}}(\theta)\right)\left(I_{n_\delta} \otimes \psi_d(\theta)\right) = I_{n_\delta} \otimes \psi_d^{\mathrm{T}}(\theta) \psi_d(\theta) = \underbrace{\psi_d^{\mathrm{T}}(\theta) \psi_d(\theta)}_{>0} I_{n_\delta}. \tag{S45}
$$

Then for all $t \geqslant t_e$ the following inequality holds:

$$
V_f(t) \geqslant \underbrace{\underline{\mathcal{M}_{\psi_d}^2} \Delta_{\min}^2 \alpha e^{-\sigma(t_e - t_\epsilon)} \psi_d^{\mathrm{T}}(\theta) \psi_d(\theta)}_{>0} I_{n_\delta} \geqslant \sqrt[n_\delta]{\underline{\mathcal{M}_{x\delta 0}}} I_{n_\delta}, \tag{S46}
$$

from which, $\forall t \geqslant t_e$, $|\mathcal{M}_{x\delta 0}| \geqslant \underline{\mathcal{M}_{x\delta 0}} > 0$, which completes the proof of Lemma 2. ■

## III. Proof of Theorem in the Manuscript

***Theorem 1.*** *Let Assumptions 1 and 2, condition (16) and Hypotheses (17)-(19) be met, then, if $\overline{\varphi}(t) \in \mathrm{FE}$ and $\left(h_\delta^{\mathrm{T}} \Phi_\delta(t) \otimes I_n\right) \in \mathrm{FE}$, the observer (24), (25) ensures that the goal (5) is achieved and additionally guarantees that:*

$$
\begin{gathered}
\lim_{t \to \infty} \left\|\tilde{x}_{\delta 0}(t)\right\| = 0\,(\exp), \ \lim_{t \to \infty} \left\|\tilde{\kappa}(t)\right\| = 0\,(\exp), \lim_{t \to \infty} \left\|\tilde{T}_I(t)\right\| = 0 \ (\exp), \\
\lim_{t \to \infty} \left\|\hat{U}(t) - U(t)\right\| = \lim_{t \to \infty} \left\|\tilde{U}(t)\right\| = 0 \ (\exp).
\end{gathered}
$$

*Proof:* The state observation error equation $\tilde{x}(t) = \hat{x}(t) - x(t)$ is written:

$$
\begin{aligned}
&\tilde{x}(t) = \hat{T}_I(t) \hat{\xi}(t) - T_I(t) \xi(t) \pm \hat{T}_I(t) \xi(t) = \hat{T}_I(t) \left(\hat{\xi}(t) - \xi(t)\right) + \left(\hat{T}_I(t) - T_I(\theta)\right) \xi(t) = \\
&= \hat{T}_I(t) \left(\hat{\xi}(t) - \xi(t)\right) + \tilde{T}_I(t) \xi(t) \pm T_I(\theta) \left(\hat{\xi}(t) - \xi(t)\right) = \\
&= \tilde{T}_I(t) \left(\hat{\xi}(t) - \xi(t)\right) + \tilde{T}_I(t) \xi(t) + T_I(\theta) \left(\hat{\xi}(t) - \xi(t)\right) = \\
&= \tilde{T}_I(t) \left(\hat{R}^{\mathrm{T}}(t) \hat{\kappa}(t) - R^{\mathrm{T}}(t) \kappa(\theta)\right) + \tilde{T}_I(t) \xi(t) + T_I(\theta) \left(\hat{R}^{\mathrm{T}}(t) \hat{\kappa}(t) - R^{\mathrm{T}}(t) \kappa(\theta)\right) = \\
&= \tilde{T}_I(t) \left(\hat{R}^{\mathrm{T}}(t) \hat{\kappa}(t) - R^{\mathrm{T}}(t) \kappa(\theta) \pm R^{\mathrm{T}}(t) \hat{\kappa}(t)\right) + \tilde{T}_I(t) \xi(t) + \\
&+ T_I(\theta) \left(\hat{R}^{\mathrm{T}}(t) \hat{\kappa}(t) - R^{\mathrm{T}}(t) \kappa(\theta) \pm R^{\mathrm{T}}(t) \hat{\kappa}(t)\right) =
\end{aligned} \tag{S47}
$$

$$
\begin{aligned}
&= \tilde{T}_I(t)\left(\tilde{R}^{\mathrm{T}}(t)\hat{\kappa}(t) + R^{\mathrm{T}}(t)\tilde{\kappa}(t) \pm \tilde{R}^{\mathrm{T}}(t)\kappa(\theta)\right) + \tilde{T}_I(t)\xi(t) + \\
&+ T_I(\theta)\left(\tilde{R}^{\mathrm{T}}(t)\hat{\kappa}(t) + R^{\mathrm{T}}(t)\tilde{\kappa}(t) \pm \tilde{R}^{\mathrm{T}}(t)\kappa(\theta)\right) = \\
&= \tilde{T}_I(t)\left(\tilde{R}^{\mathrm{T}}(t)\tilde{\kappa}(t) + R^{\mathrm{T}}(t)\tilde{\kappa}(t) + \tilde{R}^{\mathrm{T}}(t)\kappa(\theta)\right) + \tilde{T}_I(t)\xi(t) + \\
&+ T_I(\theta)\left(\tilde{R}^{\mathrm{T}}(t)\tilde{\kappa}(t) + R^{\mathrm{T}}(t)\tilde{\kappa}(t) + \tilde{R}^{\mathrm{T}}(t)\kappa(\theta)\right) = \\
&= \tilde{T}_I(t)\left(\tilde{U}^{\mathrm{T}}(t)\tilde{x}_{\delta 0}(t) + R^{\mathrm{T}}(t)\tilde{\kappa}(t) + \tilde{U}^{\mathrm{T}}(t)x_{\delta 0}(t)\right) + \tilde{T}_I(t)\xi(t) + \\
&+ T_I(\theta)\left(\tilde{U}^{\mathrm{T}}(t)\tilde{x}_{\delta 0}(t) + R^{\mathrm{T}}(t)\tilde{\kappa}(t) + \tilde{U}^{\mathrm{T}}(t)x_{\delta 0}(t)\right).
\end{aligned}
$$

where $\hat{R}^{\mathrm{T}}(t) - R^{\mathrm{T}}(t) = \begin{bmatrix} 0 & 0 & \tilde{U}(t) \end{bmatrix}$.

Similarly to (S47), the disturbance observation error is obtained:

$$
\tilde{\delta}(t) = h_\delta^{\mathrm{T}}\Phi_\delta(t)\hat{x}_{\delta 0}(t) - h_\delta^{\mathrm{T}}\Phi_\delta(t)x_{\delta 0} = h_\delta^{\mathrm{T}}\Phi_\delta(t)\tilde{x}_{\delta 0}(t). \tag{S48}
$$

If Assumption 1 is met, then, as $A_K$ is a Hurwitz matrix, the following inequalities hold:

$$
\|R(t)\| \leqslant R_{\max}, \|T_I(\theta)\| \leqslant \overline{T}_I, \|\xi(t)\| \leqslant \overline{\xi}, \|x_{\delta 0}(t)\| \leqslant \overline{x}_{\delta 0}, \left\|h_\delta^{\mathrm{T}}\Phi_\delta(t)\right\| \leqslant c_{h_\delta^{\mathrm{T}}\Phi_\delta} \tag{S49}
$$

Taking (S49) into consideration, the upper bounds of (S47) and (S48) are obtained:

$$
\begin{aligned}
&\|\tilde{x}(t)\| \leqslant \left\|\tilde{T}_I(t)\right\|\left(\left\|\tilde{U}(t)\right\|\|\tilde{x}_{\delta 0}(t)\| + R_{\max}\|\tilde{\kappa}(t)\| + \left\|\tilde{U}(t)\right\|\overline{x}_{\delta 0}\right) + \left\|\tilde{T}_I(t)\right\|\overline{\xi} + \\
&+ \overline{T}_I\left(\left\|\tilde{U}(t)\right\|\|\tilde{x}_{\delta 0}(t)\| + R_{\max}\|\tilde{\kappa}(t)\| + \left\|\tilde{U}(t)\right\|\overline{x}_{\delta 0}\right), \\
&\left\|\tilde{\delta}(t)\right\| \leqslant c_{h_\delta^{\mathrm{T}}\Phi_\delta}\|\tilde{x}_{\delta 0}(t)\|,
\end{aligned} \tag{S50}
$$

from which it is concluded that the goal (5) is achieved if (26) holds, which is to be proved below.

If $\overline{\varphi}(t) \in \mathrm{FE}$ and $\left(h_\delta^{\mathrm{T}}\Phi_\delta(t) \otimes I_n\right) \in \mathrm{FE}$, then, using the results form Lemma 2, for all $t \geqslant t_e$ it holds that:

$$
|\mathcal{M}_\kappa(t)| \geqslant \underline{\mathcal{M}_\kappa} > 0,\ |\mathcal{M}_{T_I}(t)(t)| \geqslant \underline{\mathcal{M}_{T_I}} > 0,\ |\mathcal{M}_{x_{\delta 0}}(t)| \geqslant \underline{\mathcal{M}_{x_{\delta 0}}} > 0, \tag{S51}
$$

then for all $t \geqslant t_e$ the upper bounds of the solutions of the differential equations from (25) are written as:

$$
\begin{aligned}
&\|\tilde{\kappa}(t)\| \leqslant e^{-\gamma_\kappa \underline{\mathcal{M}_\kappa^2}(t-t_e)}\|\tilde{\kappa}(t_0)\|, \\
&\left\|\tilde{T}_I(t)\right\| \leqslant e^{-\gamma_{T_I}\underline{\mathcal{M}_{T_I}^2}(t-t_e)}\left\|\tilde{T}_I(t_0)\right\|, \\
&\|\tilde{x}_{\delta 0}(t)\| \leqslant e^{-\gamma_{x_{\delta 0}}\underline{\mathcal{M}_{x_{\delta 0}}^2}(t-t_e)}\|\tilde{x}_{\delta 0}(t_0)\|,
\end{aligned} \tag{S52}
$$

therefore, the errors $\tilde{\kappa}(t)$, $\tilde{x}_{\delta 0}(t)$, $\tilde{T}_I(t)$ converge exponentially to zero.

In order to prove exponential convergence of the error $\tilde{U}(t) = \hat{U}(t) - U(t)$, the following equality is written:

$$
\dot{\tilde{U}}(t) = A_K\hat{U}(t) + I_n\hat{\delta}(t) - A_K U(t) - I_n\delta(t) = A_K\tilde{U}(t) + I_n h_\delta^{\mathrm{T}}\Phi_\delta(t)\tilde{x}_{\delta 0}(t). \tag{S53}
$$

As $A_K$ is a Hurvitz matrix, the product $h_\delta^{\mathrm{T}}\Phi_\delta(t)$ is bounded according to (S49) and does not depend on the estimate $\hat{x}_{\delta 0}(t)$, then, in case $\tilde{x}_{\delta 0}(t)$ exponentially converges to zero, it is also concluded that $\tilde{U}(t)$ has the similar behavior, which together with (S52) and (S50) allows one to conclude that (26) holds and the goal (5) is achieved.

■

## IV. Description of System for Numerical Experiments

The system from the experimental section of [S5] has been considered:

$$
\begin{aligned}
\dot{x} &= \begin{bmatrix} 0 & \theta_1+\theta_2 & 0 \\ -\theta_2 & 0 & \theta_2 \\ 0 & -\theta_3 & 0 \end{bmatrix}x + \begin{bmatrix} 0 \\ 0 \\ \theta_3 \end{bmatrix}u + \begin{bmatrix} \theta_1\theta_2 \\ 0 \\ 0 \end{bmatrix}\delta, \\
y &= \begin{bmatrix} 0 & 0 & 1 \end{bmatrix}x.
\end{aligned} \tag{S54}
$$

The parameters of the exosystem (4) from the manuscript were set as:

$$
\mathcal{A}_\delta = \begin{bmatrix} 0 & 1 \\ -10 & 0 \end{bmatrix}, h_\delta^{\mathrm{T}} = \begin{bmatrix} 1 & 0 \end{bmatrix}.
$$

Being transformed into the observer canonical form (see (6), (7) in the manuscript), the system (S54) was described by the following vectors:

$$\psi_a = \begin{bmatrix} 0 \\ -(\theta_1+\theta_2+\theta_3)\,\theta_2 \\ 0 \end{bmatrix},\ \psi_b = \begin{bmatrix} \theta_3 \\ 0 \\ \theta_3\theta_2\,(\theta_2+\theta_1) \end{bmatrix},$$
$$\psi_d = \begin{bmatrix} 0 & 0 & \theta_1\theta_2^2\theta_3 \end{bmatrix}^{\mathrm{T}},$$

where $\mathcal{L}_{ab}$ was chosen such that

$$\psi_{ab}(\theta) = col\left\{-(\theta_1+\theta_2+\theta_3)\,\theta_2,\ \theta_3,\ \theta_3\theta_2\,(\theta_2+\theta_1)\right\}.$$

The condition (17) from the manuscript was satisfied for the system under consideration, and consequently, the mappings $\mathcal{S}(\psi_{ab}),\ \mathcal{G}(\psi_{ab}),\ \Pi_\theta(\Delta)$ existed and were defined as follows:

$$\mathcal{S}(\psi_{ab}) = \begin{bmatrix} \psi_{2ab}(\psi_{1ab}\psi_{2ab}+\psi_{3ab})^2 - \psi_{2ab}^4\psi_{3ab} \\ -\psi_{1ab}\psi_{2ab}-\psi_{3ab} \\ \psi_{2ab}\psi_{1ab} \end{bmatrix},$$
$$\mathcal{G}(\psi_{ab}) = diag\left\{\psi_{2ab}^3\,(\psi_{1ab}\psi_{2ab}+\psi_{3ab}),\ \psi_{2ab}^2,\ \psi_{1ab}\right\},$$
$$\Pi_\theta(\Delta) = diag\left\{\Delta^5,\ \Delta^2,\ \Delta^2\right\}.$$

In their turn, the mappings $\mathcal{T}_{\mathcal{S}}(.),\ \mathcal{T}_{\mathcal{G}}(.)$ were defined as:

$$\mathcal{T}_{\mathcal{S}}\left(\Xi_{\mathcal{S}}(\Delta)\,\mathcal{Y}_{ab}\right) = \begin{bmatrix} \mathcal{Y}_{2ab}(\mathcal{Y}_{1ab}\mathcal{Y}_{2ab}+\Delta\mathcal{Y}_{3ab})^2 - \mathcal{Y}_{2ab}^4\mathcal{Y}_{3ab} \\ -\mathcal{Y}_{1ab}\mathcal{Y}_{2ab}-\Delta\mathcal{Y}_{3ab} \\ \mathcal{Y}_{2ab}\mathcal{Y}_{1ab} \end{bmatrix},$$
$$\mathcal{T}_{\mathcal{G}}\left(\Xi_{\mathcal{G}}(\Delta)\,\mathcal{Y}_{ab}\right) = diag\left\{\begin{matrix} \mathcal{Y}_{2ab}^3\,(\mathcal{Y}_{1ab}\mathcal{Y}_{2ab}+\Delta\mathcal{Y}_{3ab}), \\ \mathcal{Y}_{2ab}^2, \\ \Delta\mathcal{Y}_{1ab} \end{matrix}\right\},$$

where

$$\Xi_{\mathcal{S}}(\Delta)\,\mathcal{Y}_{ab} = \begin{bmatrix} \mathcal{Y}_{1ab} & \mathcal{Y}_{2ab} & \mathcal{Y}_{3ab} & \Delta\mathcal{Y}_{3ab} \end{bmatrix}^{\mathrm{T}},$$
$$\Xi_{\mathcal{G}}(\Delta)\,\mathcal{Y}_{ab} = \begin{bmatrix} \mathcal{Y}_{1ab} & \mathcal{Y}_{2ab} & \Delta\mathcal{Y}_{1ab} & \Delta\mathcal{Y}_{3ab} \end{bmatrix}^{\mathrm{T}}.$$

The mapping $T_I(\theta)$ was written as follows:

$$T_I(\theta) = \begin{bmatrix} -\frac{\theta_1+\theta_2}{\theta_3} & 0 & \frac{1}{\theta_2\theta_3} \\ 0 & -\frac{1}{\theta_3} & 0 \\ 1 & 0 & 0 \end{bmatrix}.$$

In their turn, the condition (18) from the manuscript was satisfied and the mappings $\mathcal{Q}(\theta),\ \mathcal{P}(\theta),\ \Pi_{T_I}(\mathcal{M}_\theta)$ took the form:

$$\mathcal{Q}(\theta) = \begin{bmatrix} -\theta_2\,(\theta_1+\theta_2) & 0 & 1 \\ 0 & -1 & 0 \\ 1 & 0 & 0 \end{bmatrix},$$
$$\mathcal{P}(\theta) = diag\left\{\theta_2\theta_3,\ \theta_3,\ 1\right\},$$
$$\Pi_{T_I}(\mathcal{M}_\theta) = diag\left\{\mathcal{M}_\theta^2,\ \mathcal{M}_\theta,\ \mathcal{M}_\theta\right\}.$$

Therefore, the mappings $\mathcal{T}_{\mathcal{Q}}(.),\ \mathcal{T}_{\mathcal{P}}(.)$ were implemented as follows:

$$\mathcal{T}_{\mathcal{Q}}\left(\Xi_{\mathcal{Q}}(\mathcal{M}_\theta)\,\mathcal{Y}_\theta\right) = \begin{bmatrix} -\mathcal{Y}_{2\theta}\,(\mathcal{Y}_{1\theta}+\mathcal{Y}_{2\theta}) & 0 & \mathcal{M}_\theta^2 \\ 0 & -\mathcal{M}_\theta & 0 \\ \mathcal{M}_\theta & 0 & 0 \end{bmatrix},$$
$$\mathcal{T}_{\mathcal{P}}\left(\Xi_{\mathcal{P}}(\mathcal{M}_\theta)\,\mathcal{Y}_\theta\right) = diag\left\{\mathcal{Y}_{2\theta}\mathcal{Y}_{3\theta},\ \mathcal{Y}_{3\theta},\ \mathcal{M}_\theta\right\}.$$

where

$$\Xi_{\mathcal{Q}}(\mathcal{M}_\theta)\,\mathcal{Y}_\theta = \begin{bmatrix} \mathcal{Y}_{1\theta} & \mathcal{Y}_{2\theta} \end{bmatrix}^{\mathrm{T}},$$
$$\Xi_{\mathcal{P}}(\mathcal{M}_\theta)\,\mathcal{Y}_\theta = \begin{bmatrix} \mathcal{Y}_{2\theta} & \mathcal{Y}_{3\theta} \end{bmatrix}^{\mathrm{T}}.$$

Considering the vector $\psi_d(\theta)$, the condition (19) from the manuscript was satisfied, and the mappings $\mathcal{W}(\theta)$, $\mathcal{R}(\theta)$, $\Pi_{\psi_d}(\mathcal{M}_\theta)$ were written as follows:

$$\mathcal{W}(\theta) = \begin{bmatrix} 0 \\ 0 \\ \theta_1\theta_2^2\theta_3 \end{bmatrix},$$
$$\mathcal{R}(\theta) = I_3,$$
$$\Pi_{\psi_d}(\mathcal{M}_\theta) = diag\left\{1,\ 1,\ \mathcal{M}_\theta^4\right\}.$$

The transformations $\mathcal{T}_{\mathcal{W}}(.)$, $\mathcal{T}_{\mathcal{R}}(.)$ were implemented as:

$$\mathcal{T}_{\mathcal{W}}\left(\Xi_{\mathcal{W}}(\mathcal{M}_\theta)\mathcal{Y}_\theta\right) = \begin{bmatrix} 0 \\ 0 \\ \mathcal{Y}_{1\theta}\mathcal{Y}_{2\theta}^2\mathcal{Y}_{3\theta} \end{bmatrix},$$
$$\mathcal{T}_{\mathcal{R}}\left(\Xi_{\mathcal{R}}(\mathcal{M}_\theta)\mathcal{Y}_\theta\right) = diag\left\{1,\ 1,\ \mathcal{M}_\theta^4\right\},$$

where

$$\overline{\Xi}_{\mathcal{W}}(\mathcal{M}_\theta)\mathcal{Y}_\theta = \overline{\Xi}_{\mathcal{R}}(\mathcal{M}_\theta)\mathcal{Y}_\theta = \begin{bmatrix}\mathcal{Y}_{1\theta} & \mathcal{Y}_{2\theta} & \mathcal{Y}_{3\theta}\end{bmatrix}^{\mathrm{T}}.$$

## REFERENCES


[S1] Bobtsov A., Pyrkin A., Vedyakov A., Vediakova A., Aranovskiy S. "A Modification of Generalized Parameter-Based Adaptive Observer for Linear Systems with Relaxed Excitation Conditions," in IFACPapersOnLine. vol. 55, no. 12., pp.324–329, 2022.

[S2] Nikiforov V. O., "Observers of external deterministic disturbances. II. Objects with unknown parameters," Automation and Remote Control. vol. 65, no.11, pp.1724–1732, 2004.

[S3] Narendra K. S., Annaswamy A. M. Stable Adaptive Systems. Courier Corporation, 2012.

[S4] Glushchenko A., Petrov V., Lastochkin K., "Robust method to provide exponential convergence of model parameters solving linear time-invariant plant identification problem," International Journal of Adaptive Control and Signal Processing. Vol. 35. no. 6. pp. 1120–1137, 2021.

[S5] Glushchenko A., Lastochkin K., "Extended Adaptive Observer for Linear Systems with Overparameterization," in Proc. 31st Mediterranean Conference on Control and Automation (MED), pp. 789-794, 2023.
